# Supplementary material for: Enhancing Adversarial Training with Feature Separability
Source: arXiv:2205.00637 source file (2022-05-02)
Supplement: Supplementary file 1 [file appendix.tex]

\newpage
\appendix

CIFAR100 results.

\setlength{\tabcolsep}{8pt}{
\begin{table*}[]
\centering
\resizebox{\textwidth}{!}{

\begin{tabular}{@{}l|c|c|c|c|c@{}}
\hline
       & Clean & FGSM & PGD-20(8/255) & AA(8/255) & $\text{CW}_{\inf}$(8/255)     \\
\hline       
%clean + CL($\alpha/\beta = 10, \eta = 1$) &   51.27    &  36.32±0.009  & 29.55±0.001      &  28.55±0.001     & 21.40±0.002        \\
%clean + CL($\alpha/\beta = 10, \eta = 3$)            & 51.45 &    36.25±0.005 & 29.43±0.000  &    28.50±0.000          &   21.12±0.001      \\
ATFS($\alpha/\beta = 10, \eta = 1$)            & 50.44 &  35.69±0.000    &29.50±0.001  &  28.31±0.002   &   21.05±0.001         \\
ATFS($\alpha/\beta = 10, \eta = 3$)            & 48.88 &  34.76±0.005    & 28.63±0.000     &  27.44±0.001          &     20.75±0.000 \\ \hline
AT                              & 53.97 &   30.36±0.003   &   19.39±0.000    &    18.8±0.000      &  19.88±0.000      \\
AT + Auxiliary Rotation & 58.25 & 33.86±0.001 & 23.94±0.000 & 23.34±0.000 & 23.40±0.000 \\ 
TRADES($\alpha/\beta$=2.0)      &  52.06 &  28.99±0.000     &  20.34±0.001   &   19.99±0.001  &   18.21±0.001     \\
TRADES($\alpha/\beta$=5.0)      & 54.95 &   34.57±0.003     &  27.13±0.001   & 26.85±0.000&    23.43±0.000            \\
MART &    54.72     &    39.11±0.001    &   32.0±0.001     &    31.37±0.001     &   27.97±0.001\\
\hline
clean + AWP &          &       &       &   29.38         &\\
adv + AWP &    47.6  &    33.98    &   27.93    &           &\\
\hline
AT + AWP &  53.19      &   37.4±0.000    &  30.92±0.001   &   30.43±0.000        & 27.44±0.001\\
\hline
\end{tabular}
}
\caption{CIFAR100 Result on ResNet18}
\label{tab:cifar100-resnet18}
\end{table*}
}

\section{Shortcomings of Features Learned by Existing Adversarial Training Algorithms. }
\label{sec:featureshortcoming}

\section{Implementation of ATFS + AWP}
\label{sec:ATFSAWP}
ATFS + AWP

\section{Feature Visualization}
\label{sec:featurevisualization}

\begin{figure}[h]
\centering
\subfloat{\includegraphics[width = 0.25\textwidth]{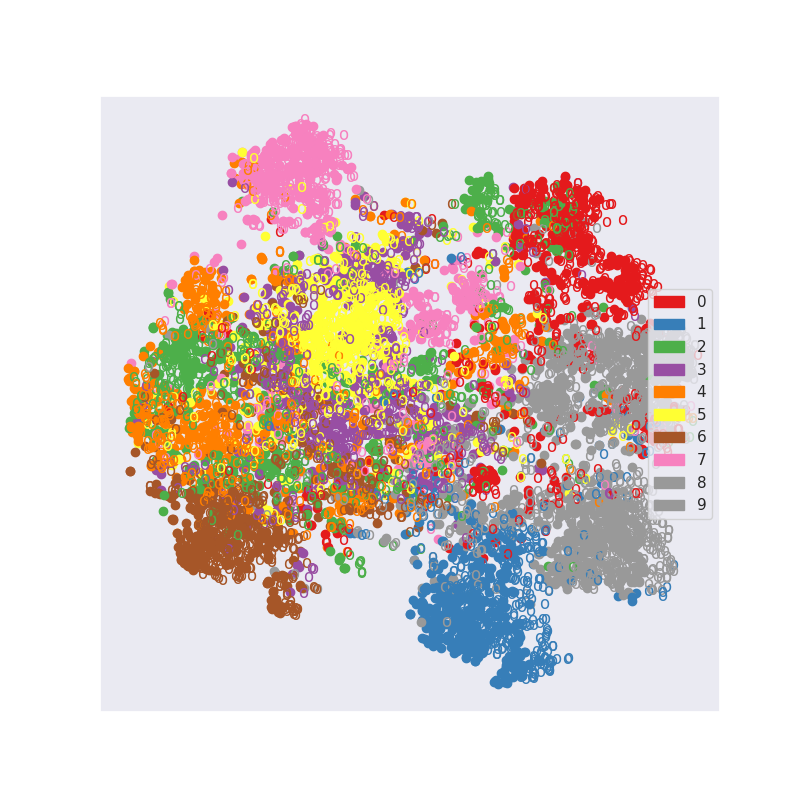}} 
\caption{The left figure shows the feature space t-SNE visualization for standard adversarial training model, the right figure shows the feature space for ATFS.}
\label{fig:similairty}
\end{figure}
